# Supplementary material for: CEV-LM: Controlled Edit Vector Language Model for Shaping Natural Language Generations
Source: arXiv:2402.14290 source file (2024-02-22)
Supplement: Supplementary file 1 [file other_attrs.tex]

\section{Evaluating on Other Attributes}
\label{appendix:other_attrs}

\input{sections/tables/delta_tab_other_attr}
\input{sections/tables/sim_tab_other_attrs}
